# Supplementary material for: Graphene-Based Platform for Infrared Near-Field Nanospectroscopy of Water and Biological Materials in an Aqueous Environment
Source: arXiv:1509.01743 source file (2015-09-05)
Supplement: Supplementary file 1 [file SI_ACSnano.pdf]

# *Supporting Information*

# Graphene-based Platform for Infrared Near-Field Nano-Spectroscopy of Water and Biological Materials in an Aqueous Environment

O. Khatib[1,2], J. D. Wood[3,4,5,6], A. S. McLeod[1], M. D. Goldflam[1], M. Wagner[1], G. L. Damhorst[6,7], J. C. Koepke[4,5,6], G. P. Doidge[4,5,6], A. Rangarajan[4,5,6], R. Bashir[4,6,7], E. Pop[8], J. W. Lyding[4,5,6], M. H. Thiemens[1], F. Keilmann[9], and D. N. Basov[1]

[1]*Dept. of Physics, Univ. of California, San Diego, La Jolla, CA 92093, USA*
[2]*Dept. of Physics, Dept. of Chemistry, and JILA, Univ. of Colorado, Boulder, CO 80309, USA*
[3]*Dept. of Materials Science and Engineering, Northwestern Univ., Evanston, IL 60208, USA*
[4]*Dept. of Electrical and Computer Engineering, Univ. of Illinois at Urbana-Champaign, Urbana, IL 61801, USA*
[5]*Beckman Institute for Advanced Science and Technology, Univ. of Illinois at Urbana-Champaign, Urbana, IL 61801, USA*
[6]*Micro and Nanotechnology Laboratory, Univ. of Illinois at Urbana-Champaign, Urbana, IL 61801, USA*
[7]*Dept. of Bioengineering, Univ. of Illinois at Urbana-Champaign, Urbana, IL 61801 USA*
[8]*Dept. of Electrical Engineering, Stanford Univ., Stanford, CA 94305, USA*
[9]*Ludwig-Maximilians-Universität and Center for Nanoscience, 80539 München, Germany*

* To whom correspondence should be addressed: Omar.Khatib@Colorado.edu

**Contents:**

- **Section S1: Materials and Methods**
  - *I. Graphene Growth and Transfer*
  - *II. Tobacco Mosaic Virus (TMV) Deposition*
  - *III. High Pressure Environment*
- **Figure S1: Scanning electron microscopy (SEM) images of a graphene/TMV/graphene nanosandwich**
- **Figure S2: Atomic force microscopy (AFM) imaging of a graphene-encapsulated TMV**

**Section S1. Materials and Methods**

*I. Graphene Growth and Transfer*

We grew graphene using chemical vapor deposition (CVD) on Cu foil (Alfa Aesar) following previously established procedures.[1, 2] For bottom graphene layers in bilayer samples, we used our conventional poly(methyl methacrylate) (PMMA) transfer method,[3, 4] followed by a forming gas ($Ar/H_2$, 4:1) anneal for 90 min at 400 °C. We employed this transfer process to produce the bottom graphene layers for the samples on $SiO_2$ (see Figs. 3 and 4). We rinsed all transferred samples in three 18.2 MΩ·cm DI $H_2O$ baths for 15 min each.

For all other graphene layers (Figs. 2, 3, 4, etc.), we needed to minimize the amount of topside residue, as this residue would obscure our imaging. Therefore, we transferred our graphene lids with poly(bisphenol A carbonate) (PC) scaffold,[2] which was removed by chloroform soaking overnight (at least 12 hr). This process obviated the need for an $Ar/H_2$ forming gas anneal. By Raman spectroscopy, we observed no interlayer chloroform intercalation in our transfer protocol.

To place the graphene lids on TMV/mica or on TMV/G/$SiO_2$ samples, we wet transferred PC-supported graphene on the biomolecule-graphene stacks. This wet transfer introduced $H_2O$ at the interface[3, 5] of the graphene and its biomolecule impregnated substrate. We removed excess $H_2O$ by spinning the samples on a spin coater at 3000 RPM for 60 s. We repeated this procedure if the sample appeared wet optically, as determined by an absence of a PC- or PMMA-related rainbow pattern. We note that this process does not completely remove $H_2O$—just the excess—thereby providing an aqueous environment for infrared (IR) spectroscopic interrogation of biomolecules.

*II. Tobacco Mosaic Virus (TMV) Deposition*

Tobacco mosaic viruses (TMV) were purified from TMV-infected tobacco plants (courtesy of Sadia Bekal, Dept. of Agricultural and Biological Engineering, University of Illinois at Urbana-Champaign). In brief, TMV were removed from infected tobacco leaves via sedimentation and centrifugation.[5] After centrifugation, a murky white supernatant was extricated. We deposited 10 to 40 μL of this concentrated TMV solution onto our annealed graphene sheets on $SiO_2$/Si (300 nm, SQI) or on freshly cleaved, bare mica (V-1 grade, SPI). We incubated the TMV droplets for 5 min, after which we blew the samples dry with $N_2$. Then, we rinsed the sample five times in 18.2 MΩ·cm DI $H_2O$. We then either imaged the sample or transferred a graphene layer over the deposited TMV, as aforementioned.

*III. High Pressure Environment*

Water trapped between graphene layers has been shown to produce high a hydrostatic pressure (ca. 1 GPa) that counters the adhesion forces between graphene sheets.[5, 6] The discussed protocol for removing excess $H_2O$ via centripetal acceleration can be tuned by the angular

velocity. Preliminary evidence suggests that the amount of $H_2O$ removed can be modified by the angular velocity used. In particular, high angular velocities (>6000 RPM) lead to isolated, $H_2O$ filled bubbles. These bubbles are separated by what appear, via atomic force microscopy, to be dry graphene/graphene regions. Lower angular velocities (ca. 3000 RPM) produce the high hydrostatic pressure environments shown in the manuscript. We therefore hold that lower hydrostatic pressures which better mimic true biological environments are achievable with proper processing conditions.

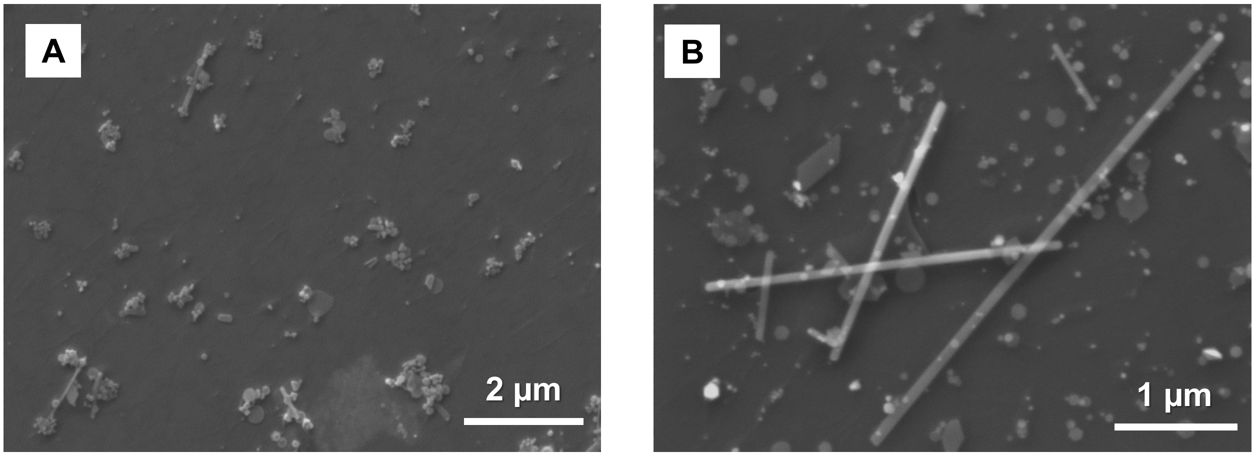


**Figure S1. Scanning electron microscopy (SEM) images of a graphene/TMV/graphene nanosandwich.** Low magnification **(A)** and high magnification **(B)** images of graphene-encapsulated TMV on graphene/mica. Residual tobacco plant matter (rectangular features) and stacked TMV are clearly contrasted in the graphene nanosandwich. The two graphene layers greatly lower the charging and electron beam damage that would otherwise affect the TMV.

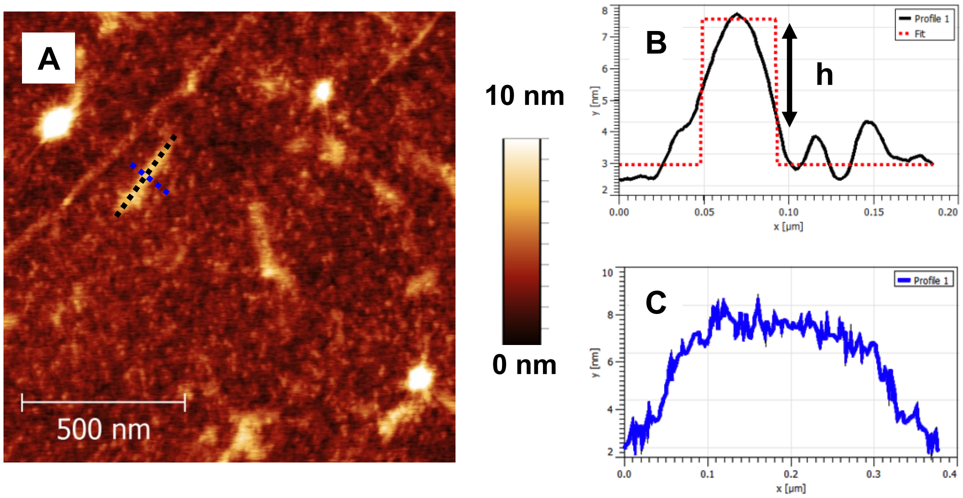


**Figure S2. Atomic force microscopy (AFM) imaging of a graphene-encapsulated TMV. (A)** AFM height image of TMV virions on graphene/mica encapsulated by another graphene layer. The rod-shaped TMV are evident under the graphene overlayer, with $H_2O$ tendrils and graphene wrinkles also present. Height profiles **(B)** perpendicular and **(C)** along the selected virion in (A). The virion's height has been decreased by the graphene overlayer to $h = 4.6 \pm 0.5$ nm (17 points averaged). As seen in (C), the virion's capsid relatively homogeneous, despite the graphene-induced hydrostatic pressure.

**References**

1. Wood, J. D.; Schmucker, S. W.; Lyons, A. S.; Pop, E.; Lyding, J. W. *Nano Letters* **2011,** 11, (11), 4547-4554.

2. Wood, J. D.; Doidge, G. P.; Carrion, E. A.; Koepke, J. C.; Kaitz, J. A.; Datye, I.; Behnam, A.; Hewaparakrama, J.; Aruin, B.; Chen, Y.; Dong, H.; Haasch, R. T.; Lyding, J. W.; Pop, E. *Nanotechnology* **2015,** 26, 055302.

3. He, K. T.; Wood, J. D.; Doidge, G. P.; Pop, E.; Lyding, J. W. *Nano Letters* **2012,** 12, (6), 2665-2672.

4. Koepke, J. C.; Wood, J. D.; Estrada, D.; Ong, Z.-Y.; He, K. T.; Pop, E.; Lyding, J. W. *ACS Nano* **2013,** 7, (1), 75-86.

5. Wood, J. D. "Large-Scale Growth, Fluorination, Clean Transfer, and Layering of Graphene and Related Nanomaterials," Ph.D. thesis. University of Illinois at Urbana-Champaign, Urbana, IL, 2013.

6. Algara-Siller, G.; Lehtinen, O.; Wang, F. C.; Nair, R. R.; Kaiser, U.; Wu, H. A.; Geim, A. K.; Grigorieva, I. V. *Nature* **2015,** 519, (7544), 443-445.
